# Supplementary material for: Byzantine-Resilient Population Protocols
Source: arXiv:2105.07123 source file (2024-02-04)
Supplement: Supplementary file 1 [file appendix.tex]

\section{Second Algorithm Termination}

Next, is the lemma for termination.

\begin{lemma}
For $n > e^{24}$ and $f < n / c_1$, 
if in the final phase at least $n/8$ honest nodes have the same value $\psi \in \{A,B\}$,
while the remaining honest nodes have no value,
then with probability at least $1 - 1/n$ all honest nodes will decide value $\psi$.
\end{lemma}

\begin{proof}
During the final phase 
a honest node $u$ participates in $z = c_1 \ln^2 n$ exchanges.
During these exchanges it counts the number of nodes that have a value.
At the end it picks the value with the highest count tally.

Without loss of generality assume that the majority value is $v = A$.
During this final phase the honest nodes will not change their values due to exchanges with faulty nodes.
Only faulty nodes may pretend to hold value $b$.

The probability that an exchange that includes $v$ is with one of the at least $n/8$ nodes
is at least $(n/8) / n = 1 / 8$.
Thus, the count $X$ of value $A$ by node $v$ has expected value 
at least $\mu = c_1 \ln^2 n \cdot 1/8$.
From Lemma \ref{lemma:chernoff}, 
for $c_1 \geq 16$ and $\delta = 1/2$,
the probability that the count $X$ is at most $\ln^2 n \leq \mu/2 = (1 - \delta) \mu$,
is less than $e^{-\delta^2 \mu / 2} \leq e^{-2 \ln^2 n} \leq n^{-2 \ln n}$.
Therefore,
the probability that the count of $A$ is at most $\ln^2 n$ in any of the honest nodes 
is at most $n \cdot n^{-2 \ln n} \leq n^{-1}$.
Thus, with probability at least $1 - 1/n$, all honest nodes will have a count of at least $\ln^2 n$,
for the value $A$.

For $f \leq n / (4 c_1) $, 
the probability that an exchange that includes $v$ is with one of the $f$ faulty nodes
is $f/n \leq 1 / (4 c_1)$.
Thus, the count $Y$ of value $B$ by node $v$ has expected value 
at most $\mu = c_1 \ln^2 n \cdot 1 / (4 c_1) = (\ln^2 n) / 4$.
From Lemma \ref{lemma:chernoff},
for $\delta = 1$, 
the probability that the count $Y$ is at least $(\ln^2 n) / 2 \geq 2 \mu$,
is at most $e^{-\delta^2 \mu / 3} = e^{- \ln^2 n / 12} = n^{-\ln n / 12} < n^{-2}$.
Therefore, from the union bound the count of $Y$ in every node will not exceed $(\ln^2 n) / 2$
with probability at least $1 - 1/n$.

Combining the above two results and their respective probabilities,
we obtain the result as needed.
\end{proof}

\section{Randomized Algorithm}

Let $a_0$ and $a_1$ be the number of honest nodes that have initial value $0$ and $1$, respectfully.
Let $a_{z_{\max}} - a_{z_{\min}} \geq 4 f$, 
where $z_{\max} \in \{0,1\}$ and $z_{\min} = 1 - z_{\max}$ 
are the respective majority and minority values amongst the honest nodes.

Initially the total difference between majority and minority among honest nodes is $d = 4f$. 
After the first cancellation phase the difference between the
the majority and minority amongst the honest nodes may decrease to $d = 4f - f = 3f$,
since $f$ honest nodes with the value $z_{\max}$ may have been convinced by Byzantine nodes 
to cancel their value by pretending to hold the minority value in exchanges. 
After the first duplication phase the difference may become $d = 2 \cdot 3f - f = 5f$,
since $f$ additional honest nodes may have been convinced to adopt the minority value $z_{\min}$.
Similarly, at the end of the second cancellation phase the difference becomes $5f - f = 4f$,
and at the end of the second duplication phase the difference becomes $2 \cdot 4f - f = 7f$.

Generalizing,
denote by $d'_i$ and $d_i$ the difference at the end of the 
respective $i$th cancellation and duplication phases.
Let $d_0 \geq 4f$ (the initial difference).
From the discussion above,
For $i > 0$, $d'_i \geq d_{i-1} - f$,
and $d_i \geq 2 d'_i - f  \geq 2 (d_{i-1} - f) - f = 2 d_{i-1} - 3f$.
When solving the recurrence,
we get for $i > 1$: 
$$
d_i = 2^i d_0 - 3f \sum_{j=0}^{i-1} 2^j
\geq 2^i 4f -3f (2^i - 1) = 2^i f + 3f = (2^i + 3)f.
$$
